# Supplementary material for: Fuzzy Tiling Activations: A Simple Approach to Learning Sparse Representations Online
Source: arXiv:1911.08068 source file (2021-03-16)
Supplement: Supplementary file 1 [file appendix-lta-gradient.tex]

\subsection{LTA Gradient Analysis}\label{lta-gradient}

In this section, we address potential doubts about the gradient issues when using LTA in a neural network. We first 

\subsubsection{Gradient inference}

Based on your request to check gradient inference, we show the figure here. We consider three measures for gradient interference. Let $l_\theta$ be the DQN loss parameterized by $\theta$. Given two random samples (i.e. experiences) $X, X'$ from ER buffer, we estimate %$\nabla_\theta l_\theta (X)^\top \nabla_\theta l_\theta (X')$, this is saying on average, did we generalize positively or did we interfere? 

\newcommand{\EE}{\mathbb{E}}
\begin{enumerate}
	\item m1: $\EE[\nabla_\theta l_\theta (X)^\top \nabla_\theta l_\theta (X')]$, this is to measure on average, whether the algorithm generalizes positively or interfere. %This is shown in Figure~\ref{fig:discrete-control-graddot}.
	%\item m2: $\nabla_{\tilde{\theta}} l_\theta (X)^\top \nabla_{\tilde{\theta}} l_\theta (X')$, where $\tilde{\theta}$ means those parameters in the second hidden layer. This is shown in Figure~\ref{fig:discrete-control-graddot}
	%\item m2: $|\nabla_\theta l_\theta (X)^\top \nabla_\theta l_\theta (X')|$, this is kind of a harsh criterion, we consider any different directions as interference and measure average orthogonality. 
	\item m2: $\EE[\nabla_\theta l_\theta (X)^\top \nabla_\theta l_\theta (X')]$ ONLY for those pairs of gradient vectors who have negative inner product. This is to check for those likely interfered gradient directions, how much they interfere with each other.
	 %This is shown in Figure~\ref{fig:discrete-control-neggraddot}.
	\item m3: Within a minibatch of pairs of $(X, X')$, the proportion of negative gradient inner products (i.e. if $32$ out of $64$ pairs has negative inner products, then the proportion is $50\%$). This is to roughly check how likely it is to get conflict gradient directions by randomly drawing two experiences from ER buffer.
\end{enumerate}

\iffalse
\begin{figure*}[!htbp]
	%		\vspace{-0.3cm}
	\centering
\subfigure[Acrobot (v1)]{
	\includegraphics[width=\figwidthfour]{figures/Acrobot-v1__graddot}}
\subfigure[MountainCar (v0)]{
	\includegraphics[width=\figwidthfour]{figures/MountainCar-v0__graddot}}
\subfigure[CartPole (v1)]{
	\includegraphics[width=\figwidthfour]{figures/CartPole-v1__graddot}}
\subfigure[LunarLander (v2)]{
	\includegraphics[width=\figwidthfour]{figures/LunarLander-v2__graddot}}
%\	%\begin{minipage}{\figwidththree}
\caption{
	Measure m1. % All algorithms are trained without using target networks. %For each point in the learning curve, we randomly draw $64$ samples from the ER buffer to estimate the interference. %The learning curve is smoothed over a window of size $10$ before averaging across runs. 
}\label{fig:discrete-control-graddot}
\end{figure*}

\begin{figure*}[!htbp]
	%		\vspace{-0.3cm}
	\centering
	\subfigure[Acrobot (v1)]{
		\includegraphics[width=\figwidthfour]{figures/Acrobot-v1__neggraddot2ndlayer}}
	\subfigure[MountainCar (v0)]{
		\includegraphics[width=\figwidthfour]{figures/MountainCar-v0__neggraddot2ndlayer}}
	\subfigure[CartPole (v1)]{
		\includegraphics[width=\figwidthfour]{figures/CartPole-v1__neggraddot2ndlayer}}
	\subfigure[LunarLander (v2)]{
		\includegraphics[width=\figwidthfour]{figures/LunarLander-v2__neggraddot2ndlayer}}
	%\	%\begin{minipage}{\figwidththree}
	\caption{
		Measure m2. %All algorithms are trained without using target networks. %For each point in the learning curve, we randomly draw $64$ samples from the ER buffer to estimate the interference. %The learning curve is smoothed over a window of size $10$ before averaging across runs. 
	}\label{fig:discrete-control-neggraddot}
\end{figure*}
\fi

It should be noted that we normalize the gradient vectors to unit length before computing inner product. For each point in the learning curve, we randomly draw $64$ samples from the ER buffer to estimate the interference. 

\begin{figure*}[!htbp]
	%		\vspace{-0.3cm}
	\centering
		\subfigure[m1]{
		\includegraphics[width=\figwidththree]{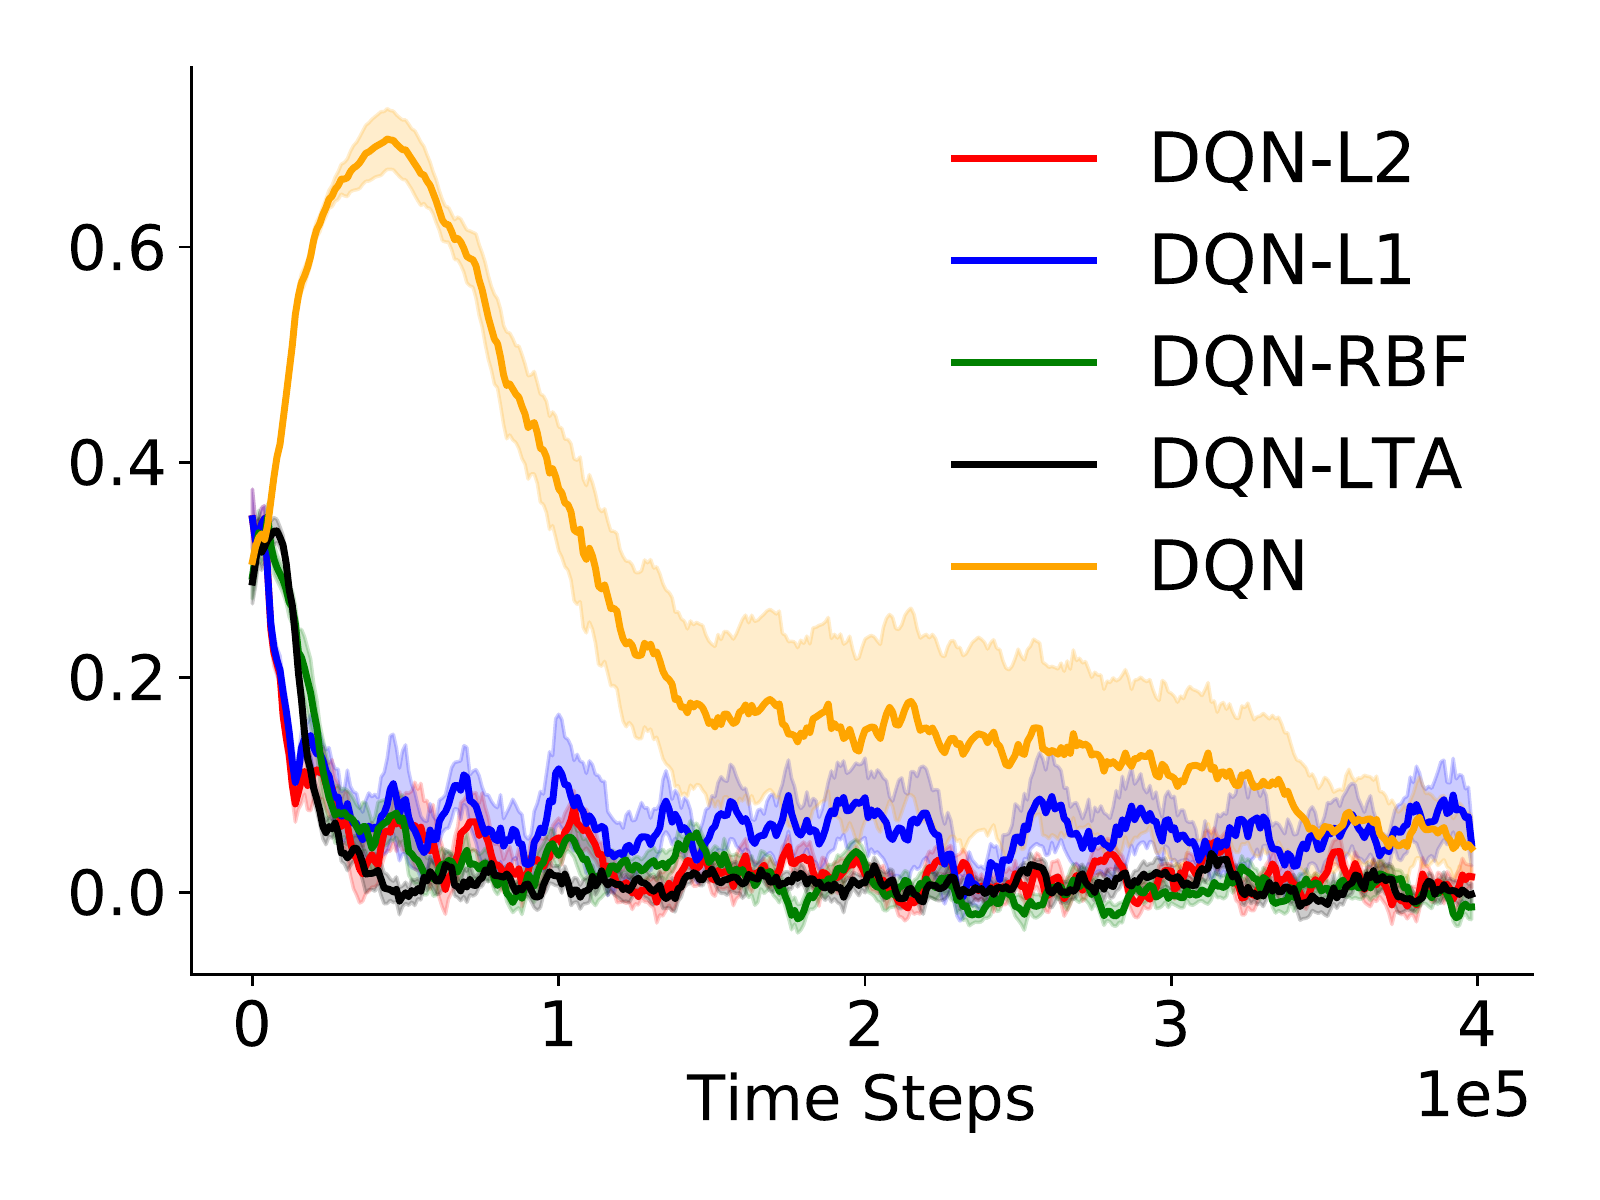}}
	\subfigure[m2]{
		\includegraphics[width=\figwidththree]{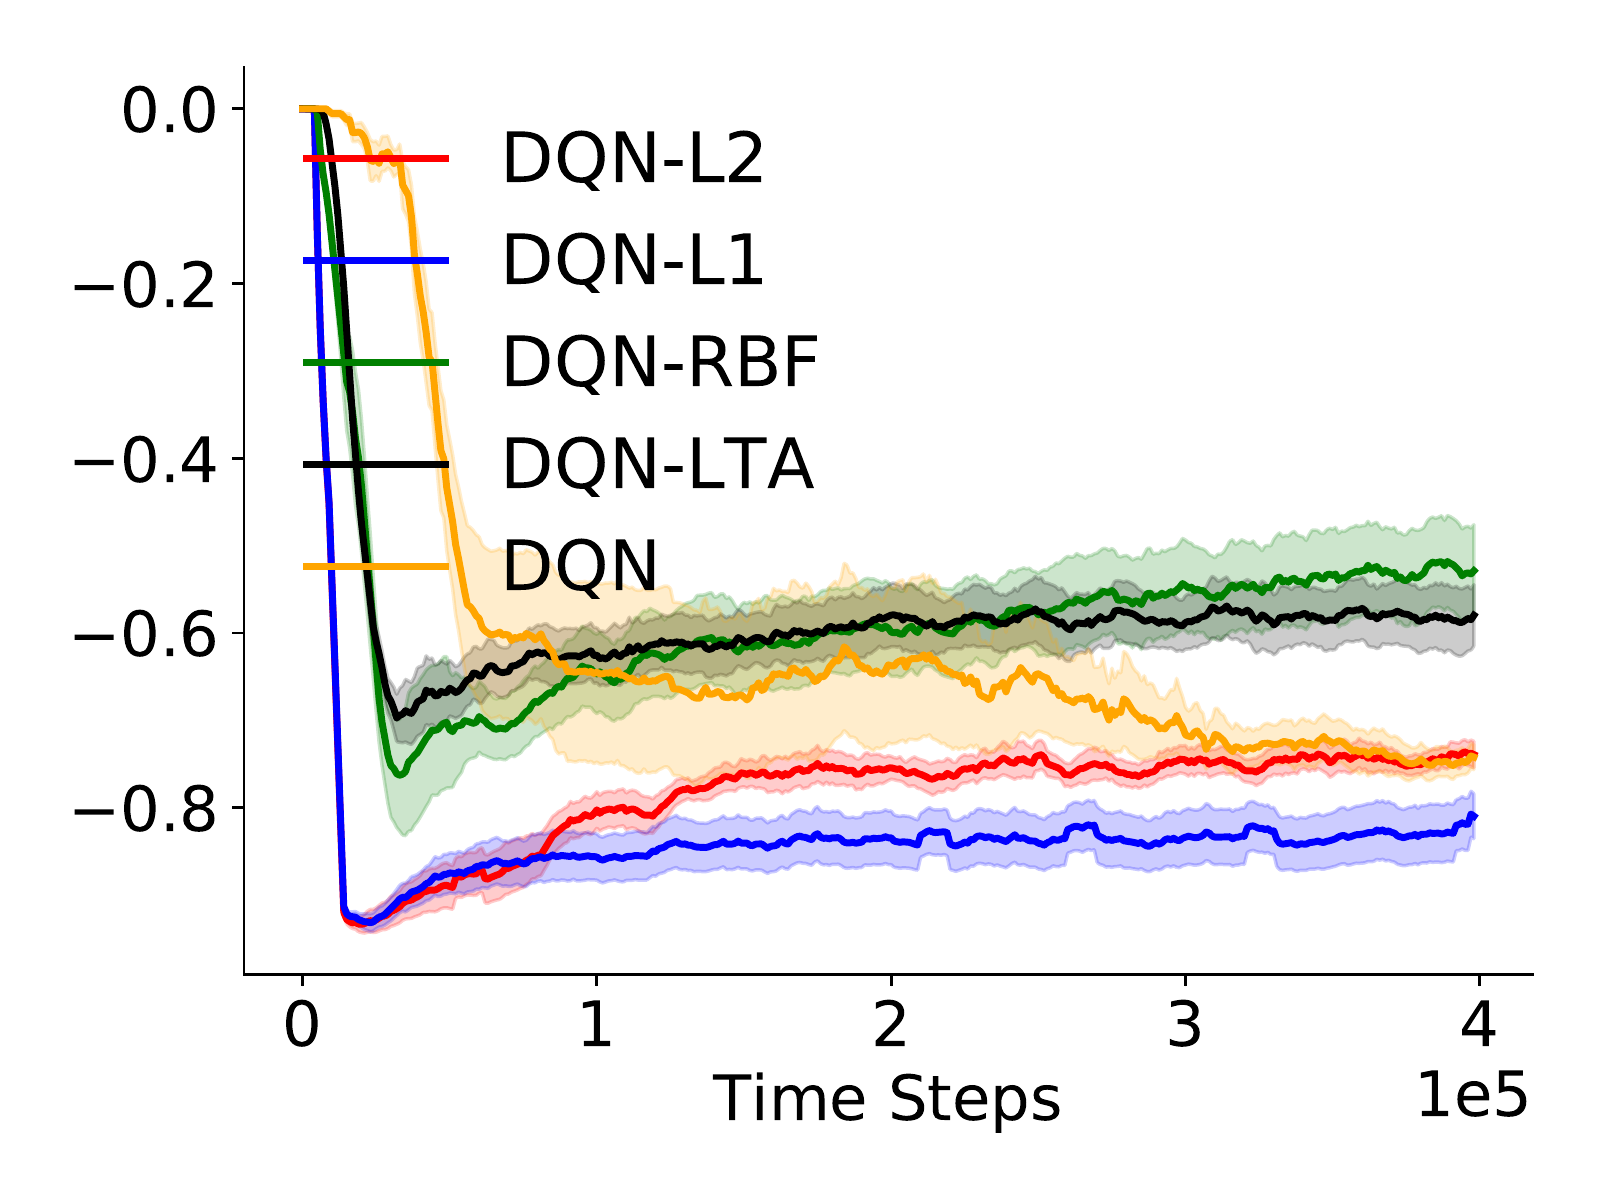}}
	\subfigure[m3]{
	\includegraphics[width=\figwidththree]{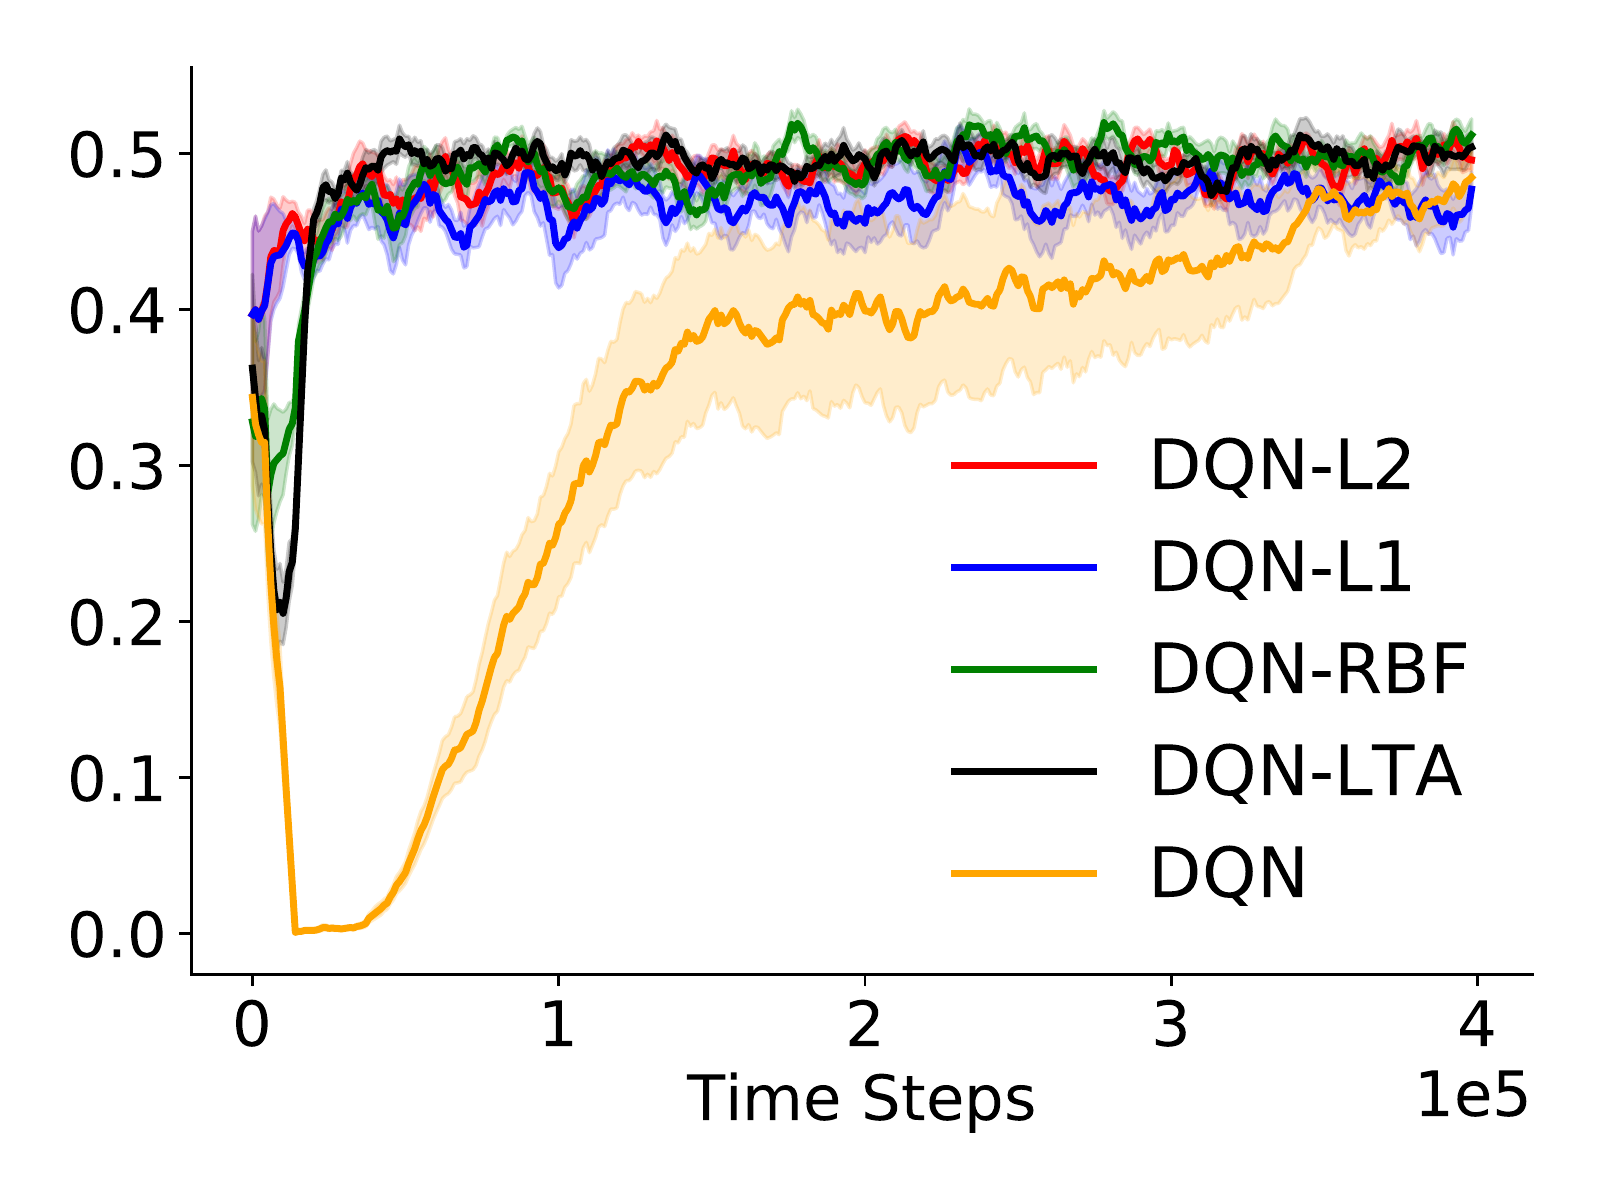}}
\\
		\subfigure[m1 in 2nd]{
		\includegraphics[width=\figwidththree]{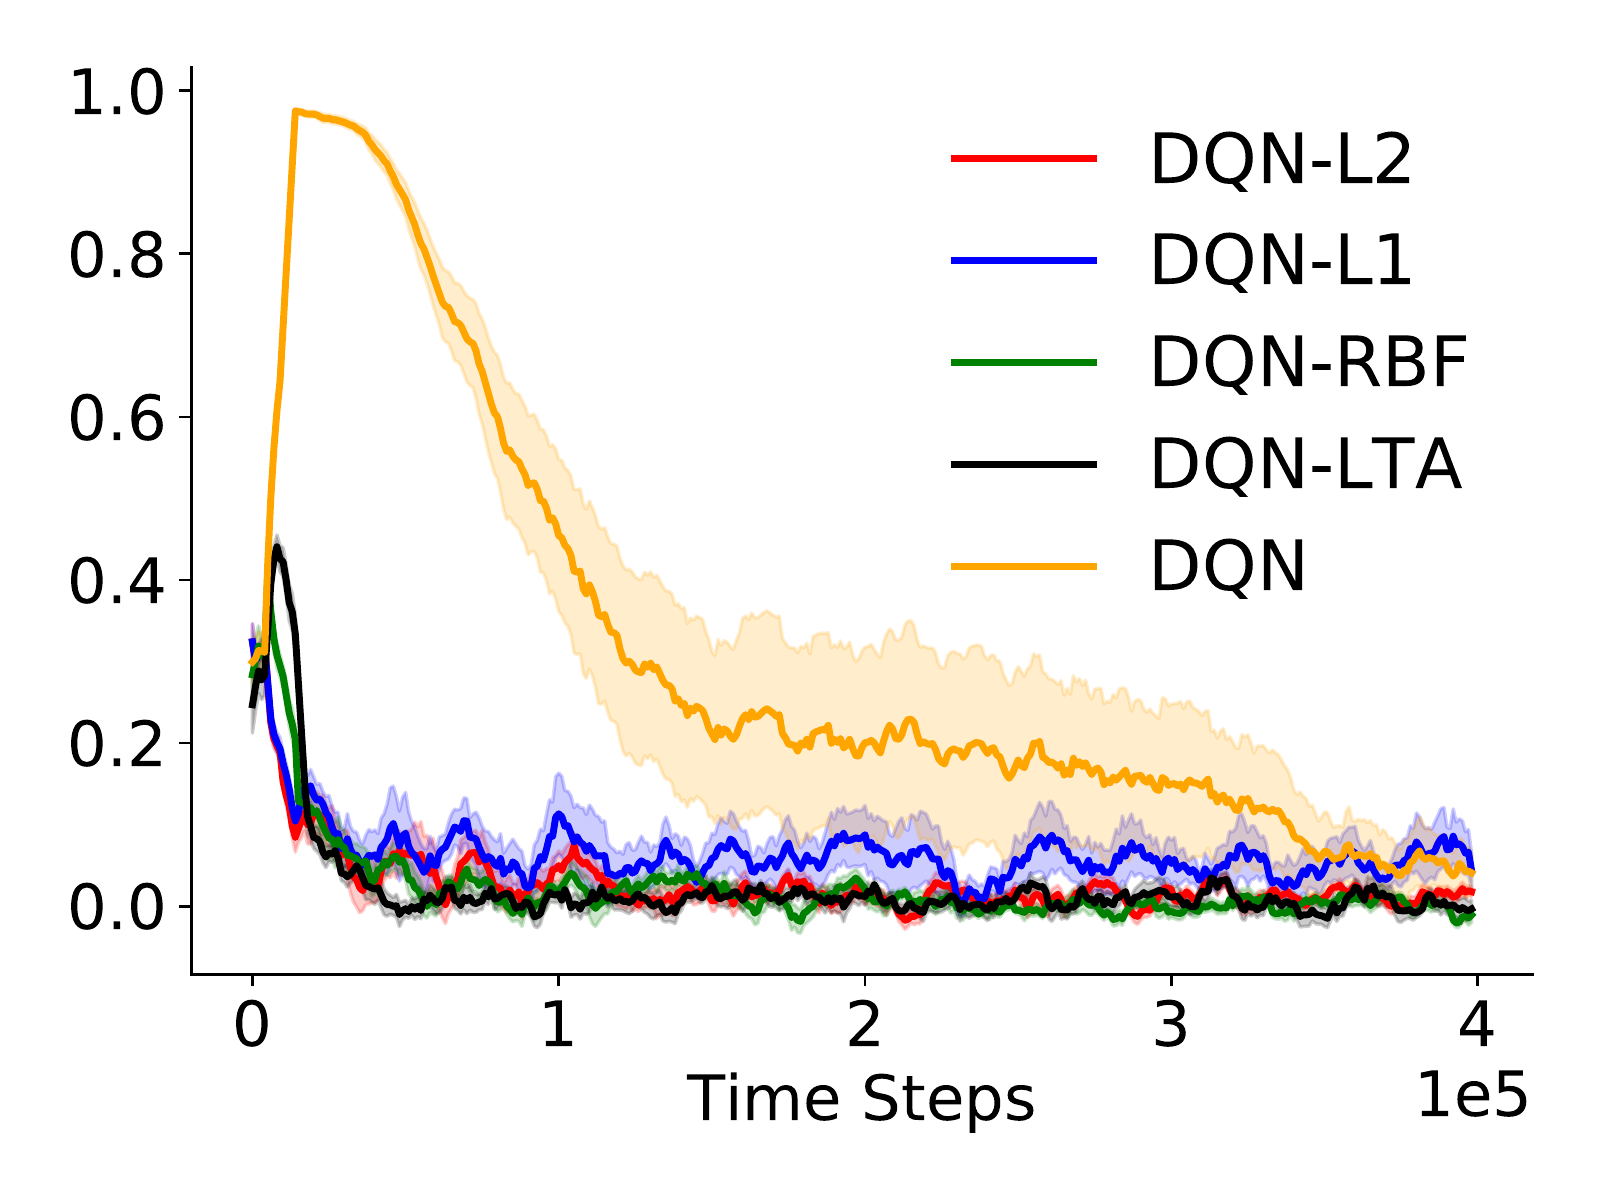}}
	\subfigure[m2 in 2nd]{
		\includegraphics[width=\figwidththree]{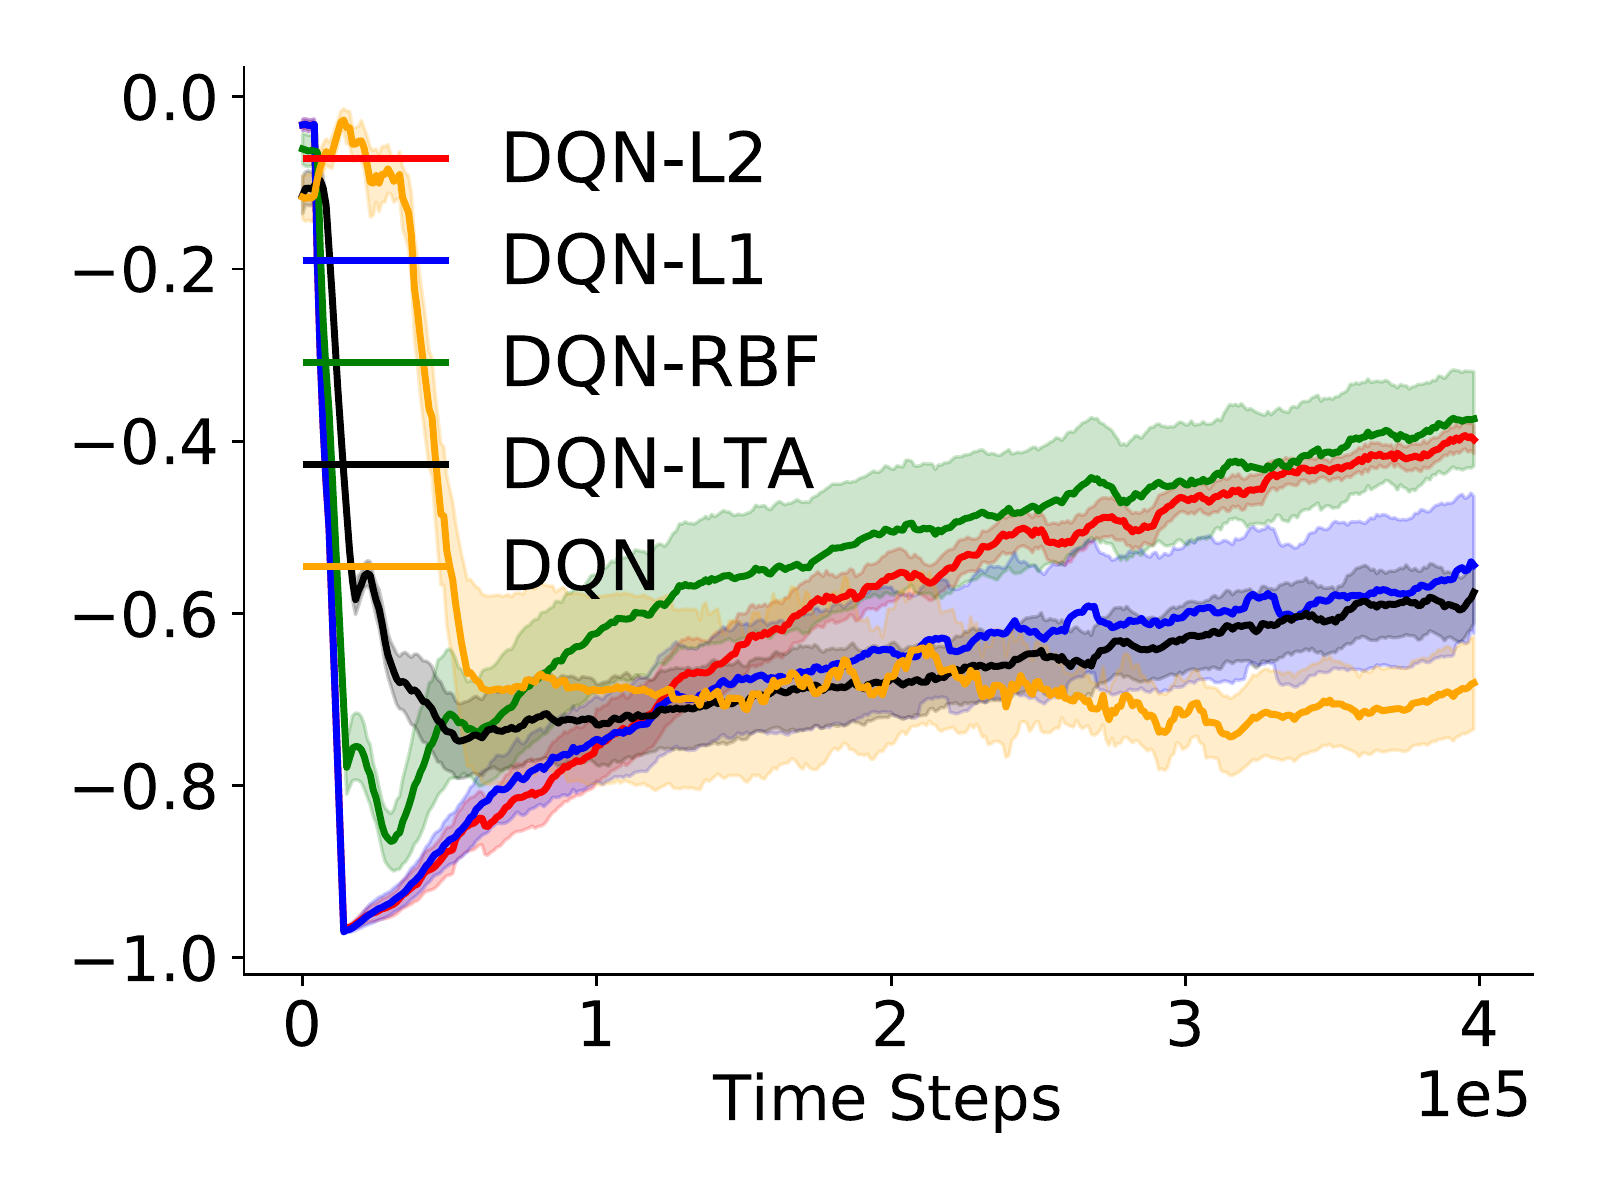}}
	\subfigure[m3 in 2nd]{
		\includegraphics[width=\figwidththree]{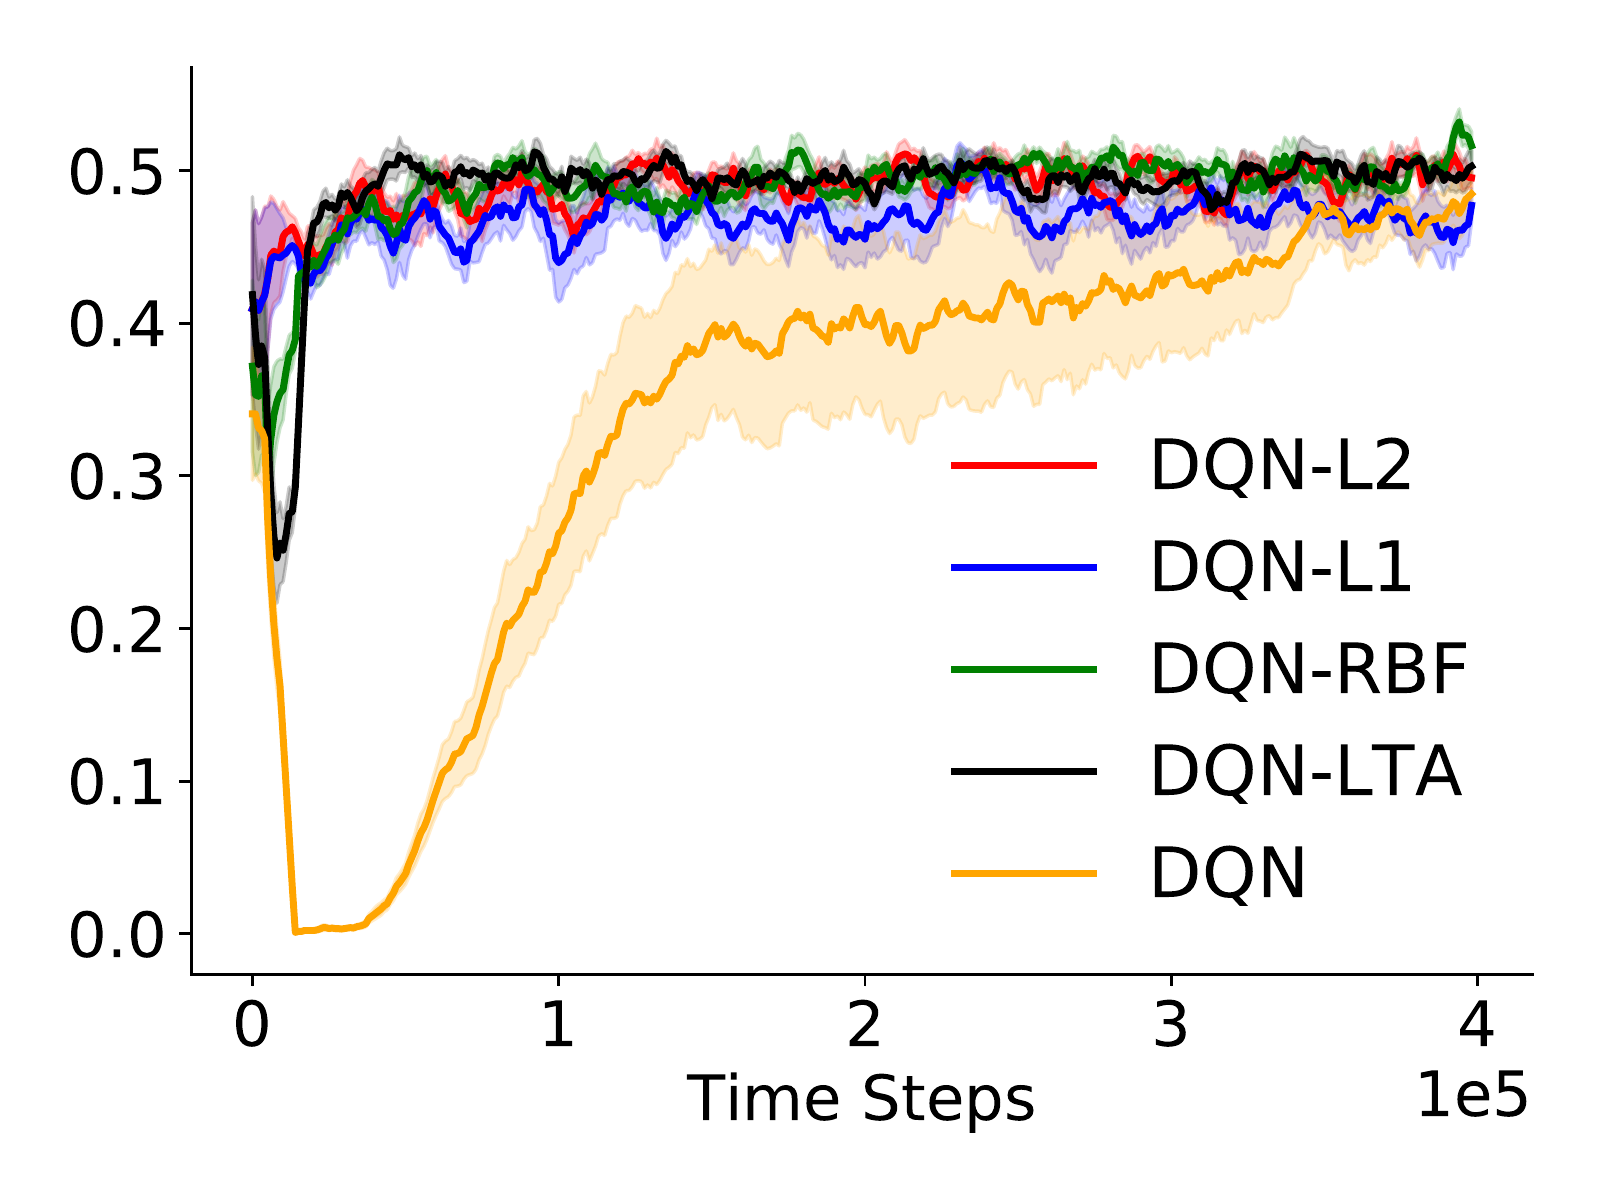}}
	%\	%\begin{minipage}{\figwidththree}
	\caption{
		Gradient inference measurements on mountain car domains, averaging over $10$ runs with the shade indicating standard error. (d)(e)(f) are measured for those parameters in the second hidden layer only (which are supposed to directly affect representation). All algorithms are trained without using target networks except DQN. The curve is smoothed over a window of size $10$ before averaging across runs. 
	}\label{fig:discrete-control-mcargrad}
\end{figure*}

\begin{figure*}[!htbp]
	%		\vspace{-0.3cm}
	\centering
	\includegraphics[width=\figwidthtwo]{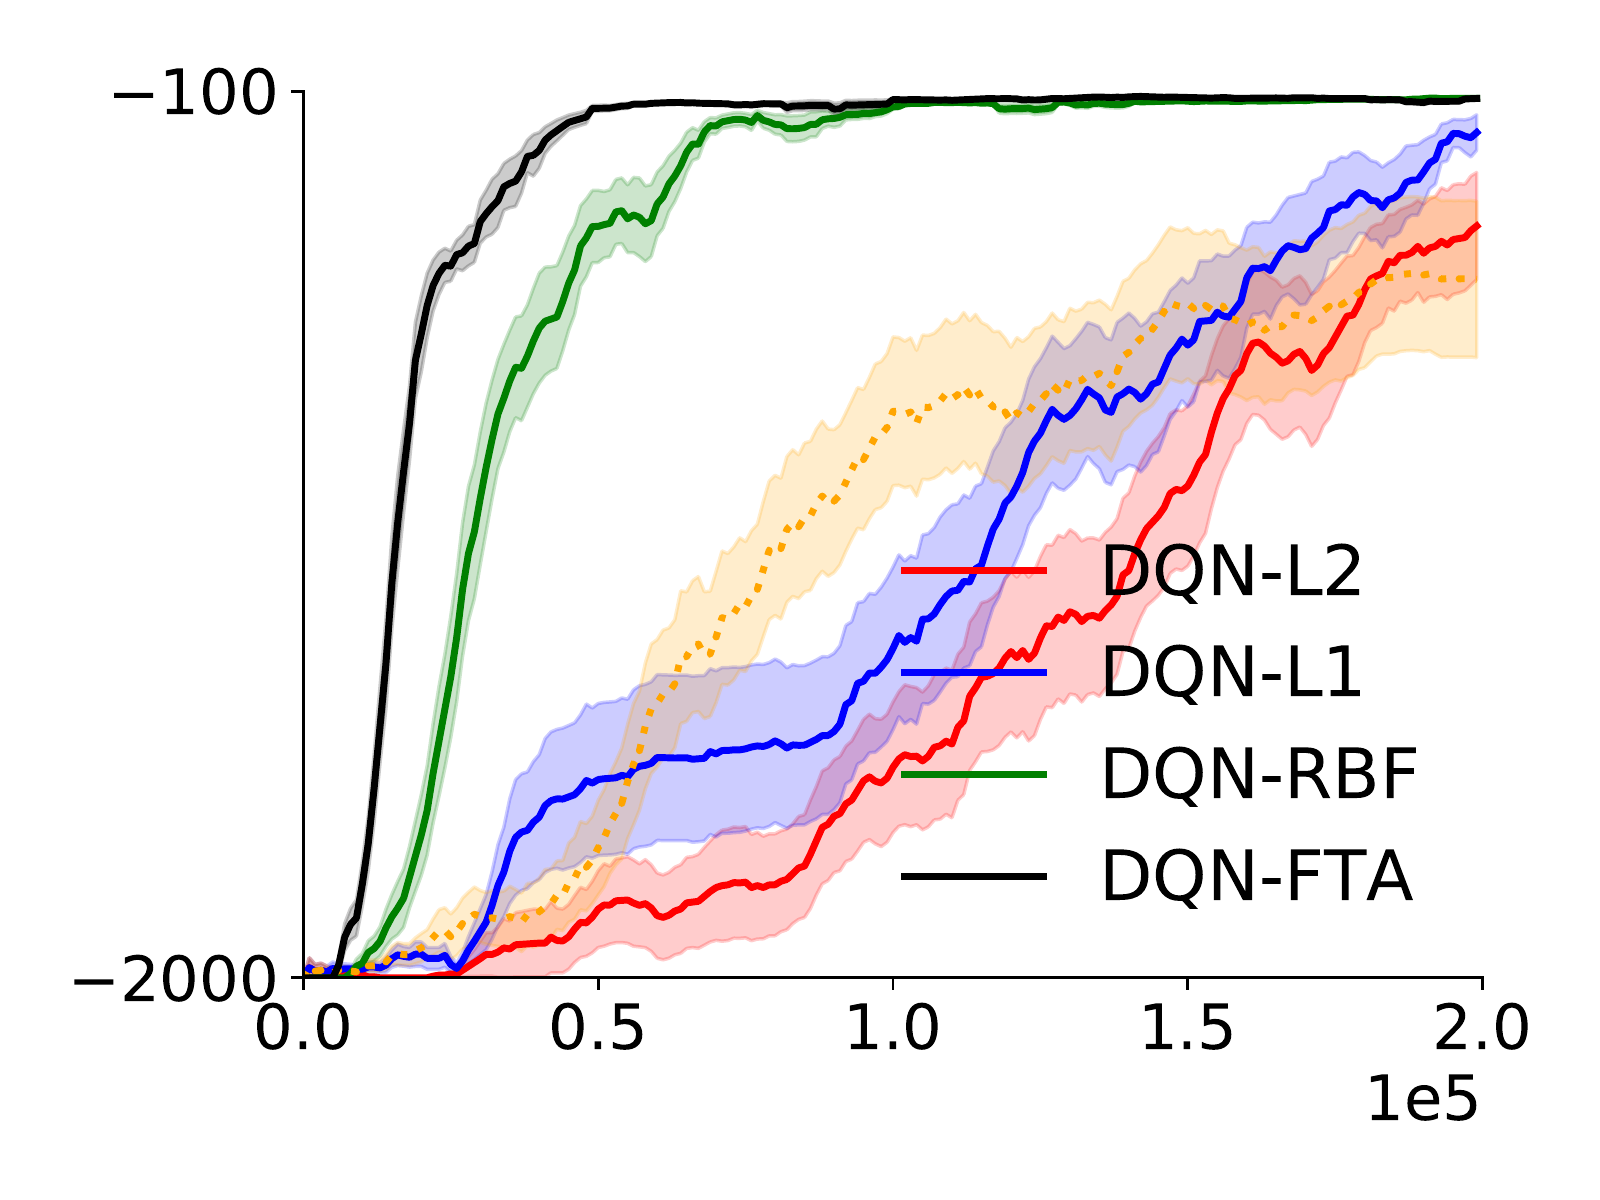}
	\caption{
		Evaluation learning curves on mountain car from our paper Figure 4(b) and 6 (b). The dotted line without label name is DQN. 
	}\label{fig:mcar-compare}
\end{figure*}

Recall that from our paper, the algorithms' performances in terms of number of time steps taken to reach optimal policy: DQN-LTA $>$ DQN-RBF > DQN-L1 $>$ DQN-L2 $\ge$ DQN (i.e. $>$ means better (use fewer time steps) and $\ge$ means slightly better). We show the learning curves of episodic returns here again in Figure~\ref{fig:mcar-compare} for convenience. 

There are several interesting observations. First, in Figure~\ref{fig:discrete-control-mcargrad}(b)(e), for the weights in the second hidden layer (m2 measurement), DQN-RBF has lower interference strength than DQN-LTA, but DQN-LTA performs better. This discrepancy indicates that it is not necessarily true that the lower interference, the better. Second, DQN tends to over generalize during early learning, which may hurt and result in bad performance. Third, figure (e) shows that DQN-L1 is similar to DQN-LTA during late learning stage in terms of m2. But DQN-L1 seems to have extremely interfered gradient directions during early learning, which may explain why it learns slower than DQN-LTA. 

These observations may indicate that DQN-LTA helps generalize \emph{appropriately}, but not overly generalize or highly interfered. We believe it is worth a separate work to thoroughly study the gradient interference issue to draw some interesting conclusions.

\subsubsection{Regarding the issue of zero gradient by using LTA}

We apologize for the possibly misleading Figure 1 for LTA in Figure 1. It uses the setting where $\eta=0.05$ or $0.1$ while $\delta=0.33$, which is actually not a good choice for visualization. We will change Figure 1 in the paper. 

Note that the sparsity control parameter $\eta$ is equal to tile width $\delta$. LTA with this setting is unlikely to give zero derivatives, and as we report empirically later, it indeed does not. Here Figure~\ref{fig:lta-visualize} visualize the LTA with $\eta=\delta=0.25$ where $\cvec=\{0, 0.25, 0.5, 0.75\}$. Note that LTA is a one-to-many (here it is $1-to-4$) mapping, any single element in the resultant $4$-dimensional output vector may pass back gradient information. 

\begin{figure*}[!htbp]
	%		\vspace{-0.3cm}
	\centering
	\includegraphics[width=\figwidthtwo]{figures/lta_delta_equal_eta}
	\caption{
		Visualization of LTA. One can see that no matter which bin $z$ hits, there is nonzero slope and the gradient information can be passed back.  
	}\label{fig:lta-visualize}
\end{figure*}

\subsubsubsection{Calculating the gradient}

We now calculate the gradients as a more rigorous treatment. Recall the following notations. 
\begin{equation}
\onehotapp(z) \defeq 1 - \indicatorplusapp(\max(\cvec-z, 0) + \max(z-\delta-\cvec, 0))
\end{equation}
where $\indicatorplusapp(x)$ will keep $x$ as whatever it is if $x<\eta$ and otherwise zero. 

Let $\xvec \in \mathbb{R}^{n_1}$ be the output from the first hidden layer and $\mathbf{W}\in \mathbb{R}^{n_1\times n_2}$ be the weights in the second hidden layer (LTA layer, in out implementation, $n_1=n_2=64$). To simplify the analysis, consider $n_2=1$ and hence $\mathbf{W}$ reduces to $\wvec \in \mathbb{R}^{n_1}$, i.e., a vector, and let's consider the gradient of the loss function w.r.t. to this weight vector. 

Also recall that we set $\eta = \delta$. 
It is sufficient to ONLY consider the case when $\xvec^\top \wvec \notin \{\cvec_1, ..., \cvec_k \}$, i.e., it does not hit any cutoff values, because during the training process, $\wvec^\top \xvec$ should be considered as a continuous random variable and the probability of it equals to certain cutoff values is zero. % We will also report empirical results later. 

Then whenever $\xvec^\top \wvec$ is between $\cvec_i, \cvec_{i+1}$ for some $i$, there must be gradient information backpropagated because $\eta=\delta>|\xvec^\top \wvec - \cvec_i| > 0$ and $\eta=\delta>|\xvec^\top \wvec - \cvec_{i+1}| > 0$. 

Specifically, after applying LTA to $\xvec^\top \wvec$, assume we have three nonzero entries (note that if we increase the value of $\eta$ there will be more nonzero entries and more gradient information will get backpropagated). After simple calculation, we can get
\[
\phi_w\defeq \onehotapp(\xvec^\top \wvec) = (0, ..., 1 - \xvec^\top \wvec + \delta + \cvec_{i-1}, 1, 1 - \cvec_{i+1} + \xvec^\top \wvec, ..., 0) \in \RR^k
\]
where $1$ value is at the $i$th position. And the square loss is $L \defeq (\phi_w^\top \theta - y)^2$ where $y$ is the training target. Let $\frac{\partial \phi_w}{\partial \wvec}$ denote the $k\times n_1$ Jacobian matrix:
\[
\frac{\partial \phi_w}{\partial \wvec} =
\left[ {\begin{array}{c}
	0 \\
	...\\
	-\xvec^\top\\
	0\\
	\xvec^\top \\
	0 \\
	...\\
	\end{array} } \right]
\]
Then
\begin{align}
\frac{\partial L}{\partial \wvec}^\top &=  \frac{\partial L}{\partial \phi_w} \frac{\partial \phi_w}{\partial \wvec} \\
&=  (\phi_w^\top \theta - y)\theta^\top \frac{\partial \phi_w}{\partial \wvec}  \\
&= (\phi_w^\top \theta - y) (\theta_{i+1} - \theta_{i-1}) \xvec^\top
\end{align}
One can see that there is no particular LTA-incurred reason leading to zero gradient. 
\\

\subsubsection{Empirical verification}

We tested that on Mountain car, when training our DQN-LTA, the proportion of parameters with nonzero gradient on the second hidden layer (LTA layer) is above $60\%$ across most of training time steps as shown in Figure~\ref{fig:mcar-gradsparse2nd}. In contrast, the activation sparsity of LTA is only about $14\%$ as we reported in our paper. We also checked that the proportion of parameters with nonzero gradient in the whole NN is above $38\%$ across most of training time steps in DQN-LTA. % Comparing with regular DQN, it seems that DQN-LTA is able to help maintain a relatively stable gradient sparsity during the whole training process. 

\begin{figure*}[!htbp]
	%		\vspace{-0.3cm}
	\centering
	\includegraphics[width=\figwidthtwo]{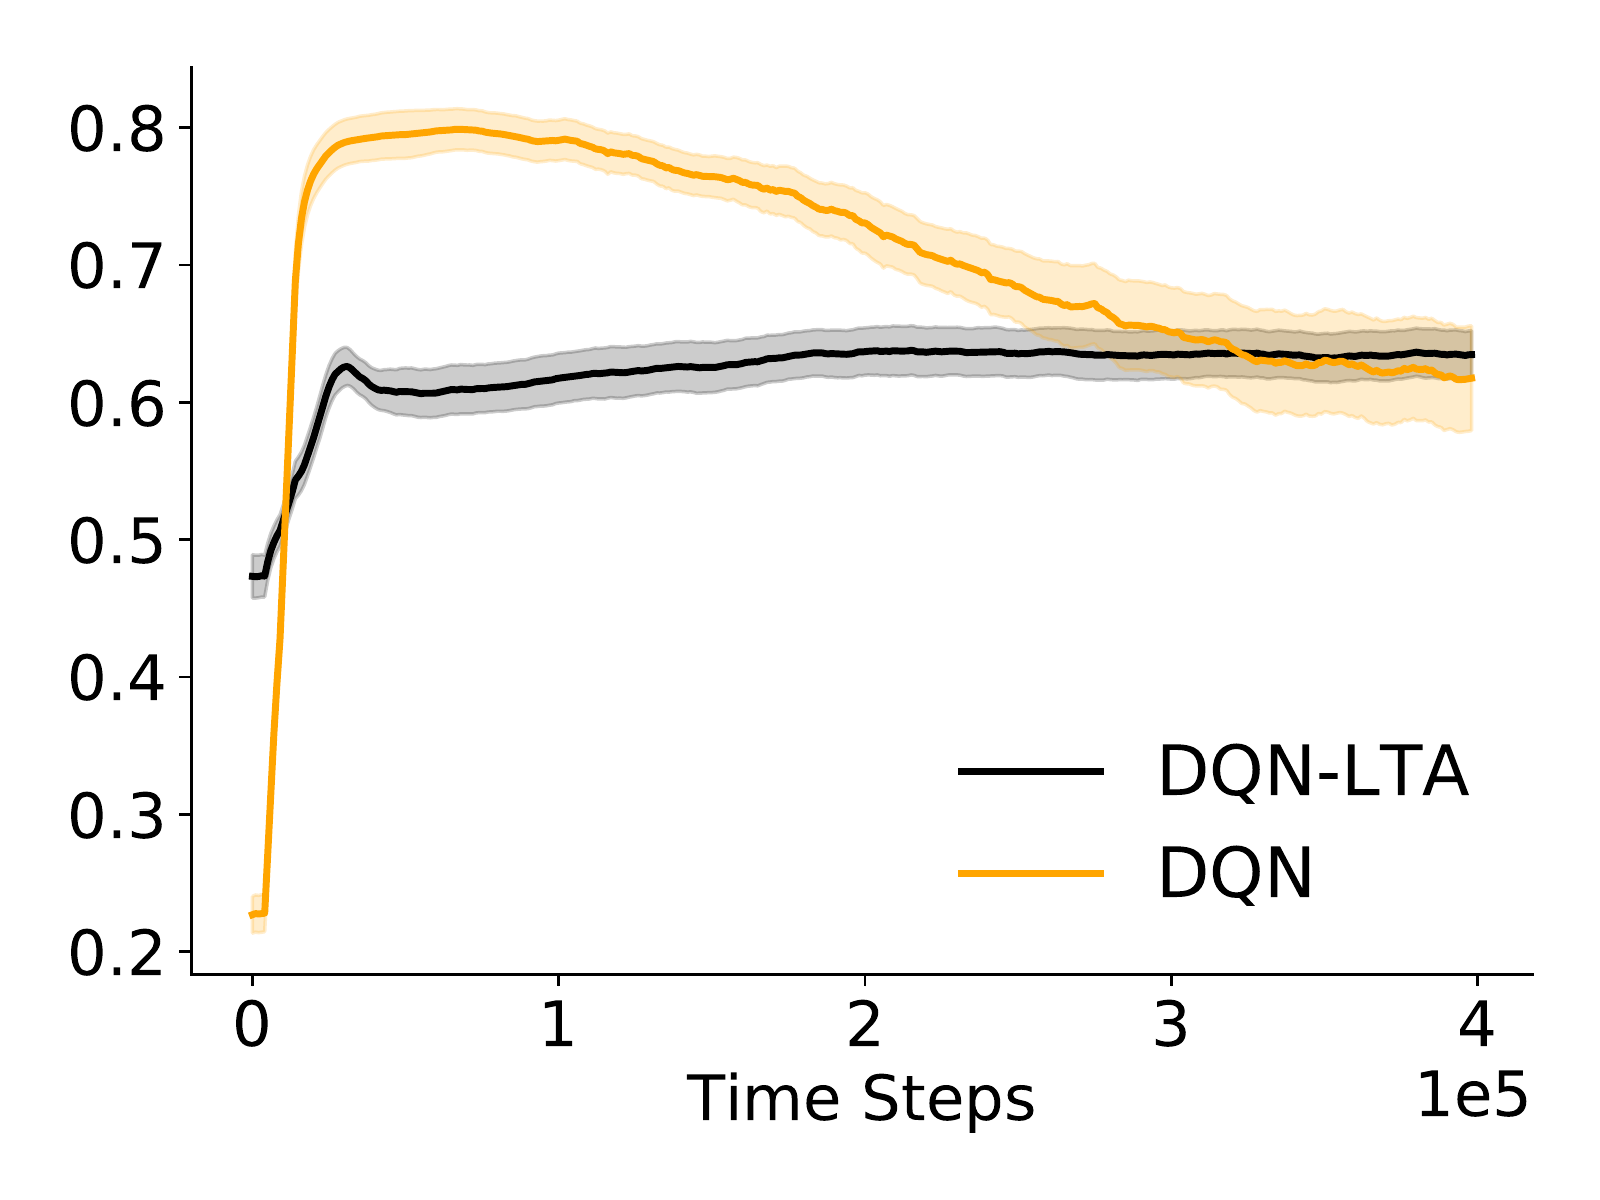}
	\caption{
		The gradient sparsity in the second hidden layer comparison between DQN-LTA and DQN. Specifically, the gradient sparsity is computed by the number of parameters with nonzero derivative in the second hidden layer divided by $64\times 64$, i.e. the number of training parameters in the second hidden layer. 
		The results are averaged over $10$ runs, and the curve is smoothed over a window of size $10$ before averaging across runs. 
	}\label{fig:mcar-gradsparse2nd}
\end{figure*}

\subsubsection{Whether we particularly tune parameter setting for LTA}

To clear your doubts, we show how DQN-L1 performance changes as we change the number of the second hidden layer units from a fine range: $\{128, 256, 384, 512, 640, 768, 896, 1024\}$ in the below Figure~\ref{fig:discrete-control-lunarsweep}. For each number of hidden units, we further optimize the regularization weight from the range $\{0.0, 0.001, 0.01, 0.1\}$. This should pose a great advantage for DQN-L1. However, recall that our DQN-LTA reaches episodic return $200$ within about $350$k environment time steps, which is significantly better than any setting of DQN-L1 here. This clearly indicates the advantage of DQN-LTA. 

\begin{figure*}[!htbp]
	%		\vspace{-0.3cm}
	\centering
		\includegraphics[width=\figwidthtwo]{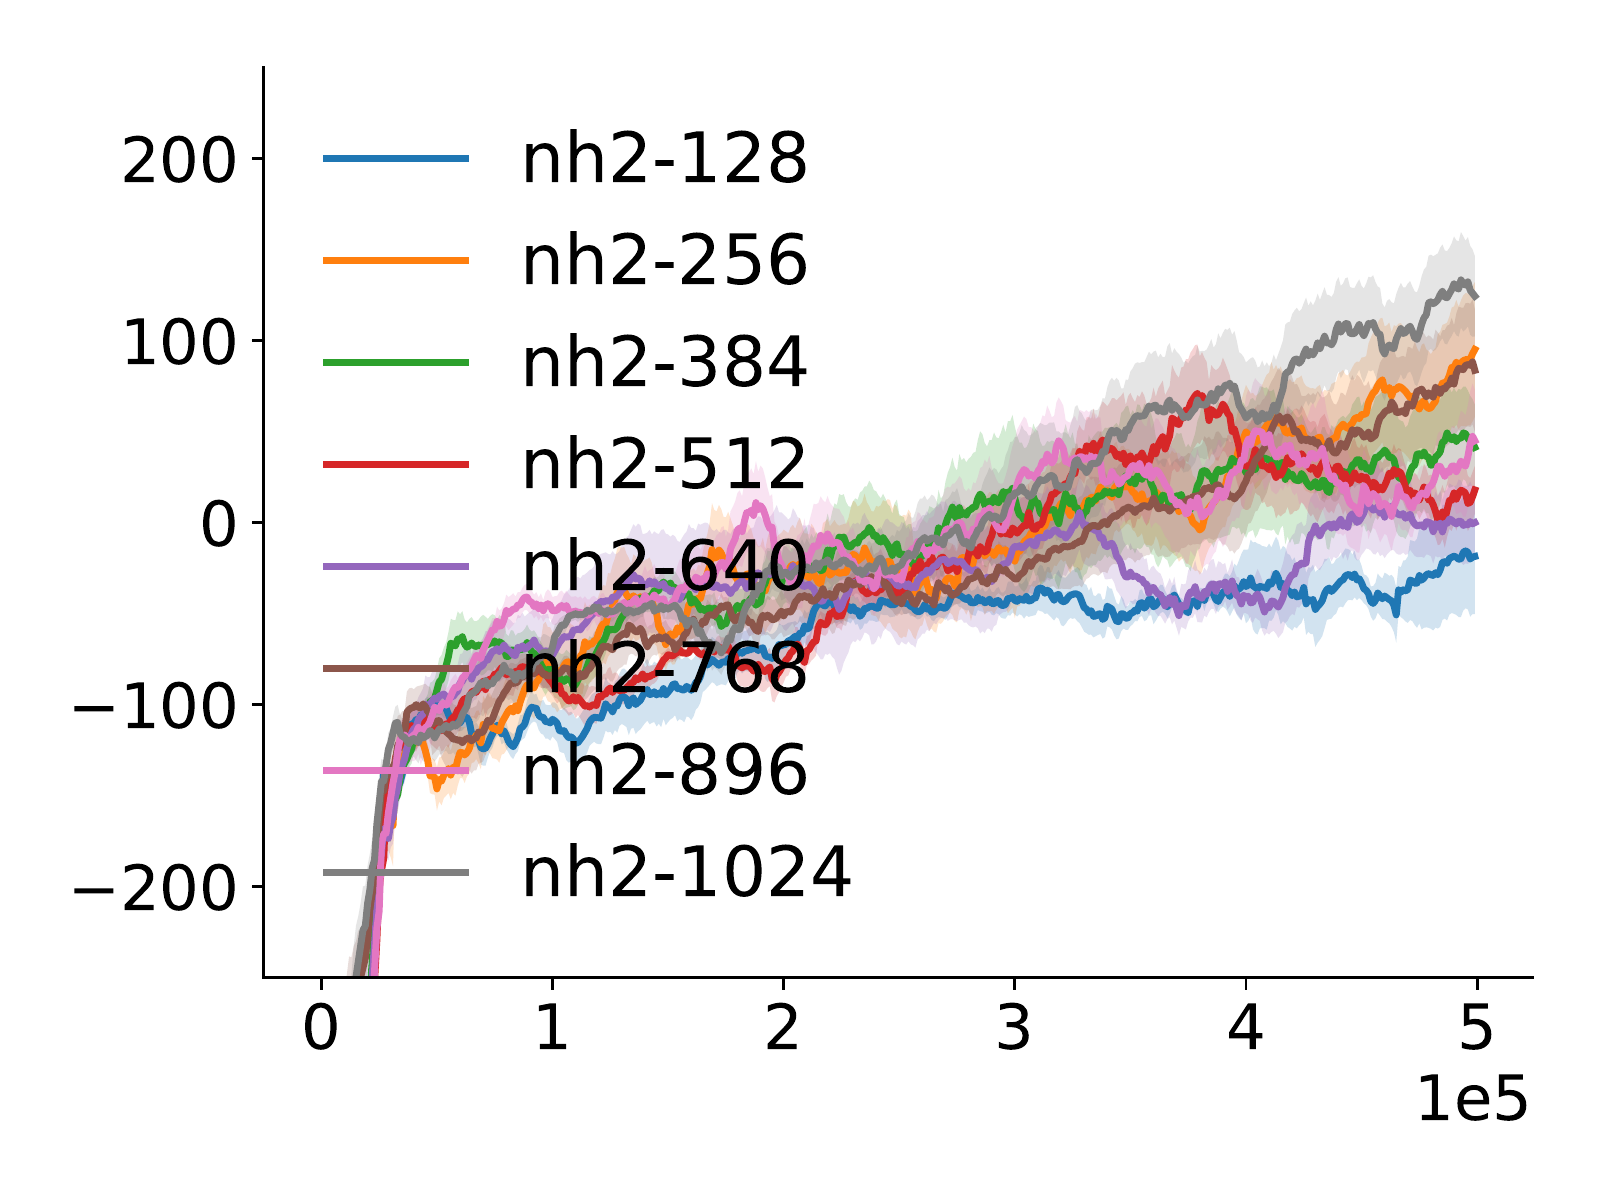}
	\caption{
		Evaluation learning curves on LunarLander, averaging over $5$ runs with the shade indicating standard error. The learning curve is smoothed over a window of size $20$ before averaging across runs. 
	}\label{fig:discrete-control-lunarsweep}
\end{figure*}
